# Supplementary material for: Levenshtein Training for Word-level Quality Estimation
Source: arXiv:2109.05611 source file (2021-09-15)
Supplement: Supplementary file 1 [file levTQE-appendix.pdf]

## A Details on Levenshtein Transformer Inference

For the  $k$ -th iteration during decoding, with source-side input  $\mathbf{x}$  and target-side sequence input  $\mathbf{y}^{(k-1)}$  of length  $J$ , suppose the decoder block output is  $\{\mathbf{h}_0, \mathbf{h}_1, \dots, \mathbf{h}_J\}$ . The following predictions and edits will take place in order:

- deletion actions  $d_j \in \mathcal{D}^{(k)}$ :

$$p_{del}^{(k)}(d_j \mid \mathbf{x}, \mathbf{y}^{(k-1)}) = \text{softmax}(\mathbf{A}_{del}^T \mathbf{h}_j)$$

for  $j \in 1 \dots J_0$  and  $J_0 = |\mathbf{y}^{(k-1)}|$

- mask insertion actions  $\gamma_j \in \mathcal{S}^{(k)}$ :

$$p_{ins}^{(k)}(\gamma_j \mid \mathbf{x}, \mathbf{y}') = \text{softmax}(\mathbf{A}_{ins}^T [\mathbf{h}_j; \mathbf{h}_{j+1}])$$

for  $j \in 0 \dots J_1$ ,  $\mathbf{y}' = \mathcal{D}^{(k)}(\mathbf{y}^{(k-1)})$  and  $J_1 = |\mathbf{y}'|$

- word prediction actions  $w_j \in \mathcal{W}^{(k)}$ :

$$p_w^{(k)}(w_j \mid \mathbf{x}, \mathbf{y}'') = \text{softmax}(\mathbf{A}_w^T \mathbf{h}_j)$$

for  $j \in 1 \dots J_2$ ,  $\mathbf{y}'' = \mathcal{S}^{(k)}(\mathcal{D}^{(k)}(\mathbf{y}^{(k-1)}))$  and  $J_2 = |\mathbf{y}''|$

In the end,  $\mathbf{y}^{(k)} = \mathcal{W}^{(k)}(\mathcal{S}^{(k)}(\mathcal{D}^{(k)}(\mathbf{y}^{(k-1)})))$ . The iterative process will continue until  $\mathbf{y}^{(k)} = \mathbf{y}^{(k-1)}$  or a maximum number of iterations is reached.

## B Details on Edit Tag Conversion to/from Subword-Level

Algorithm 1 shows the tag conversion algorithm from subword-level to word-level (for inference). Algorithm 2 shows the tag conversion algorithm from word-level to subword-level (for finetuning).

## C Details of Experimental Setup

### C.1 Data Synthesis

Here are details on how we synthesized data:

- **src-tgt-ref** We take the WMT20 en-de parallel data and translate it with the NMT system provided by the shared task organizer.
- **bt-rt-tgt** We use a 10M-sentence sample from the newscrawl2020 German monolingual data. The back-translation and the round-trip translation are performed with M2M-100-small model.

---

### Algorithm 1: Conversion of subword-level tags to word-level tags

---

**Input:** subword-level token sequence  $\mathbf{y}^{sw}$ ,  
word-level token sequence  $\mathbf{y}^w$ ,  
subword-level tag sequence  $\mathbf{q}^{sw}$

**Output:** word-level tag sequence  $\mathbf{q}^w$

$\mathbf{q}^w \leftarrow []$ ;

**for each word  $w_k$  in  $\mathbf{y}^w$  do**

    find subword index span  $(s_k, e_k)$  in  $\mathbf{y}^{sw}$   
    that corresponds to  $w_k$ ;

$\mathbf{q}_k^{sw} \leftarrow$  subword-level translation and  
    gap tags within span  $(s_k, e_k)$ ;

$g_{s_k}^{sw} \leftarrow$  subword-level gap tag before  
    span  $(s_k, e_k)$ ;      //  $g_{s_k-1}^{sw} \in \mathbf{q}^{sw}$

**if**  $\forall \mathbf{q}_k^{sw}$  are OK **then**

$\mathbf{q}^w += [g_{s_k}^{sw}, \text{OK}]$ ;

**else**

$\mathbf{q}^w += [g_{s_k}^{sw}, \text{BAD}]$ ;

**end**

**end**

$\mathbf{q}^w += [\mathbf{q}^{sw}[-1]]$ ; // add ending gap tag

**return**  $\mathbf{q}^w$ ;

---

- **src-tgt1-tgt2** We take the source side of the WMT20 en-de parallel data and translate it with the NMT system from the shared task (weaker system, tgt1) and the Facebook winning system for the WMT19 en-de news translation (Ng et al., 2019, stronger system, tgt2). We remove all the cases where tgt1 and tgt2 are identical.

### C.2 Misc.

We preprocess our data by first tokenizing with Moses tokenizer, and then applying subword segmentation. For all the LevT models without M2M-100 initialization, we use the same BPE model and source/target-side vocabulary as the official NMT checkpoint provided by the WMT20 QE shared task. For models with M2M-100 initialization, we use the M2M-100 sentencepiece model.

Under the constrained setting, we use the NMT checkpoint supplied by the shared task to generate the knowledge distillation data for LevT translation training, both for en-de and en-zh. Under the unconstrained setting, we use the Facebook winning system for the WMT19 en-de news translation.

All of our implementations are based on the Fairseq toolkit. We use the same hyperparameter for LevT translation model training as the docu-

|                                  | # sentence pairs/triplets |
|----------------------------------|---------------------------|
| shared task en-de parallel       | 23.4M                     |
| shared task en-zh parallel       | 20.3M                     |
| WMT20 en-de parallel             | 44.2M                     |
| src-tgt-ref synthetic            | 44.2M                     |
| src-tgt1-tgt2 synthetic          | 36.1M                     |
| bt-rt-tgt synthetic              | 10.0M                     |
| shared task en-de human PE train | 7K                        |
| shared task en-zh human PE train | 7K                        |
| shared task en-de human PE dev   | 1K                        |
| shared task en-zh human PE dev   | 1K                        |
| shared task en-de human PE test  | 1K                        |
| shared task en-zh human PE test  | 1K                        |

Table 4: Data Statistics for Our Experiments

ment provided in Fairseq<sup>2</sup>. For both synthetic and human post-edited data finetuning, we use Adam optimizer with a learning rate 2e-5 with warmup (4000 updates for synthetic finetuning and 2000 for human post-edited data finetuning), and we use the shared task development set to select the best checkpoint.

All the word-level and subword-level tags we use as the reference for finetuning are computed using our own TER implementation<sup>3</sup>, but we stick to the original reference tags in the test set for evaluation to avoid potential result mismatch. Our evaluations are done with the official evaluation scripts<sup>4</sup> from the shared task. The script computes the Matthews Correlation Coefficient (MCC, Matthews, 1975), which is formulated as follows:

$$S = \frac{TP + FN}{N} \quad (1)$$

$$P = \frac{TP + FP}{N} \quad (2)$$

$$MCC = \frac{TP/N - S \times P}{\sqrt{PS(1-S)(1-P)}} \quad (3)$$

where  $TP/FP$  stands for true/false positives and  $TN/FN$  stands for true/false negatives.  $N$  stands for the number of examples in the dataset. The script also computes F1 scores of the OK and BAD tags.

Table 4 shows some statistics of the data we use in our experiments.

---

#### Algorithm 2: Construction of heuristic subword-level tags

---

**Input:** subword-level token sequence  $\mathbf{y}^{sw}$ ,  
word-level token sequence  $\mathbf{y}^w$ , naive  
subword-level tag sequence  $\mathbf{q}^{sw}$ ,  
word-level tag sequence  $\mathbf{q}^w$

**Output:** heuristic subword-level tag  
sequence  $\widetilde{\mathbf{q}}^{sw}$

```

 $\widetilde{\mathbf{q}}^{sw} \leftarrow []$ ;
for each word  $w_k$  in  $\mathbf{y}^w$  do
    find subword index span  $(s_k, e_k)$  in  $\mathbf{y}^{sw}$ 
    that corresponds to  $w_k$ ;
     $\mathbf{q}_k^{sw} \leftarrow$  subword-level translation and
    gap tags within span  $(s_k, e_k)$ ;
     $t_k^w \leftarrow$  word-level translation tag for  $w_k$ ;
    //  $t_k^w \in \mathbf{q}^w$ 
     $g_k^w \leftarrow$  word-level gap tag before  $w_k$ ;
    //  $g_k^w \in \mathbf{q}^w$ 
     $\widetilde{\mathbf{q}}^{sw} += [g_k^w]$ ; // copy left gap tag
     $n = |\mathbf{q}_k^{sw}|$ ; // # subwords for  $w_k$ 
    if  $t_k^w$  is OK then
        /* word is OK, so all subwords
        and gaps between them
        should be OK */
         $\widetilde{\mathbf{q}}^{sw} += [OK] * (2n - 1)$ 
    else if  $\exists \text{BAD in } \mathbf{q}_k^{sw}$  then
        /* no conflict between
        subword-level tag and
        word-level tag - copy  $\mathbf{q}_k^{sw}$ 
        as-is */
         $\widetilde{\mathbf{q}}^{sw} += \mathbf{q}_k^{sw}$ ;
    else
        /* subword-level tag disagrees
        with word-level tag - force
        it as all-BAD to guarantee
        perfect conversion */
         $\widetilde{\mathbf{q}}^{sw} += [BAD] * (2n - 1)$ 
end
 $\widetilde{\mathbf{q}}^{sw} += [\mathbf{q}^w[-1]]$ ; // add ending gap tag
return  $\widetilde{\mathbf{q}}^{sw}$ ;

```

---

<sup>2</sup>[https://github.com/pytorch/fairseq/blob/master/examples/nonautoregressive\\_translation/README.md](https://github.com/pytorch/fairseq/blob/master/examples/nonautoregressive_translation/README.md)

<sup>3</sup>Code will be released after review.

<sup>4</sup><https://github.com/sheffieldnlp/qe-eval-scripts>
